# Supplementary material for: Self in Space: Benchmarking Self-Awareness and Spatial Cognition in UAV Embodied Intelligence
Source: arXiv:2607.12477 source file (2026-07-15)
Supplement: Supplementary file 1 [file appendix.tex]

\section{Contributions and Acknowledgments}
\label{sec:contributions}

All contributors of Seed3D 2.0 are listed in alphabetical order by their last names.

\subsection{Core Contributors}
Diandian Gu, Jing Lin, Gaohong Liu, Jiahang Liu, Su Ma, Guang Shi, Jun Wang, Qinlong Wang, Qianyi Wu, Zhongcong Xu, Xuanyu Yi, Zihao Yu, Jianfeng Zhang, Zhuolin Zheng, Yifan Zhu

\subsection{Contributors}
Rui Chen, Hengkai Guo, Xiaoyang Guo, Mingcong Han, Xu Han, Xiu Li, Yixun Liang, Weiqiang Lou, Junzhe Lu, Guan Luo, Minghan Qin, Shuguang Wang, Yuang Wang

\subsection{Acknowledgments}
Weidong Chen, Yunpeng Chen, Jinxin Chi, Zixian Du, Luyao Guo, Liang Han, Lixin Huang, Kaihua Jiang, Shihao Jiang, Yuhan Li, Huan Liu, Ziwen Ma, Wanxing Wang, Xintuo Wang, Manlian Wu, Shilong Yang, Junyang Zhang, Eddie Zhou, Jiaqing Zhou, Tong Zhou
